# Supplementary material for: Synchronization induced by external forces in modular networks
Source: arXiv:2004.00057 source file (2020-03-31)
Supplement: Supplementary file 1 [file Appendix2.pdf]

| Neuron | Index | Localization | 3 mod | Class | Ganglion | 5 mod | 10 mod |
|---|---|---|---|---|---|---|---|
| ADAL | 1 | Head | 1 | IN | E | 1 | 1 |
| ADAR | 2 | Head | 3 | IN | E | 3 | 4 |
| ADEL | 3 | Head | 2 | SN | E | 2 | 3 |
| ADER | 4 | Head | 2 | SN | E | 2 | 2 |
| ADFL | 5 | Head | 1 | SN | C | 1 | 1 |
| ADFR | 6 | Head | 3 | SN | C | 4 | 6 |
| ADLL | 7 | Head | 1 | SN | C | 1 | 1 |
| ADLR | 8 | Head | 1 | SN | C | 1 | 1 |
| AFDL | 9 | Head | 2 | SN | C | 2 | 3 |
| AFDR | 10 | Head | 2 | SN | C | 2 | 3 |
| AIAL | 11 | Head | 3 | IN | D | 4 | 6 |
| AIAR | 12 | Head | 3 | IN | D | 4 | 6 |
| AIBL | 13 | Head | 2 | IN | C | 2 | 3 |
| AIBR | 14 | Head | 2 | IN | C | 2 | 3 |
| AIML | 15 | Head | 1 | IN | D | 2 | 3 |
| AINL | 16 | Head | 3 | IN | C | 5 | 9 |
| AINR | 17 | Head | 3 | IN | C | 5 | 9 |
| AIYL | 18 | Head | 1 | IN | D | 1 | 1 |
| AIYR | 19 | Head | 1 | IN | D | 1 | 1 |
| AIZL | 20 | Head | 3 | IN | C | 3 | 9 |
| AIZR | 21 | Head | 3 | IN | C | 3 | 9 |
| ALA | 22 | Head | 1 | IN | B | 1 | 2 |
| AQR | 23 | Head | 2 | SN | E | 2 | 3 |
| ASGL | 24 | Head | 3 | SN | C | 3 | 9 |
| ASGR | 25 | Head | 3 | SN | C | 3 | 9 |
| ASHL | 26 | Head | 3 | SN | C | 3 | 8 |
| ASHR | 27 | Head | 3 | SN | C | 3 | 4 |
| ASIL | 28 | Head | 3 | SN | C | 4 | 6 |
| ASIR | 29 | Head | 3 | SN | C | 4 | 6 |
| ASKL | 30 | Head | 3 | SN | C | 3 | 4 |
| ASKR | 31 | Head | 3 | SN | C | 3 | 4 |
| AUAL | 32 | Head | 3 | IN | C | 5 | 9 |
| AUAR | 33 | Head | 3 | IN | C | 5 | 9 |
| AVAL | 34 | Head | 1 | IN | C | 1 | 1 |
| AVAR | 35 | Head | 1 | IN | C | 1 | 1 |
| AVBL | 36 | Head | 1 | IN | C | 1 | 2 |
| AVBR | 37 | Head | 1 | IN | C | 1 | 2 |
| AVDL | 38 | Head | 1 | IN | C | 3 | 7 |
| AVDR | 39 | Head | 1 | IN | C | 1 | 1 |
| AVEL | 40 | Head | 1 | IN | C | 1 | 1 |
| AVER | 41 | Head | 1 | IN | C | 1 | 1 |
| AVFL | 42 | Head | 3 | IN | E | 3 | 10 |
| AVFR | 43 | Head | 3 | IN | E | 3 | 10 |
| AVG | 44 | Head | 2 | IN | E | 2 | 3 |
| AVHL | 45 | Head | 3 | IN | C | 3 | 10 |
| AVHR | 46 | Head | 3 | IN | C | 3 | 10 |
| AVJL | 47 | Head | 1 | IN | C | 1 | 1 |
| AVJR | 48 | Head | 1 | IN | C | 1 | 1 |
| AVKL | 49 | Head | 2 | IN | D | 2 | 2 |
| AVKR | 50 | Head | 2 | IN | D | 2 | 3 |
| AVL | 51 | Head | 2 | MN | D | 2 | 3 |

| | | | | | | | |
|---|---|---|---|---|---|---|---|
| AWAL | 52 | Head | 3 | SN | C | 4 | 6 |
| AWAR | 53 | Head | 3 | SN | C | 4 | 6 |
| AWBL | 54 | Head | 3 | SN | C | 3 | 8 |
| AWBR | 55 | Head | 3 | SN | C | 3 | 8 |
| BAGL | 56 | Head | 2 | SN | A | 2 | 3 |
| BAGR | 57 | Head | 2 | SN | A | 2 | 3 |
| CEPDL | 58 | Head | 2 | SN | B | 2 | 3 |
| CEPDR | 59 | Head | 2 | SN | B | 2 | 3 |
| CEPVL | 60 | Head | 2 | SN | A | 2 | 3 |
| CEPVR | 61 | Head | 2 | SN | A | 2 | 3 |
| FLPL | 62 | Head | 1 | SN | E | 1 | 7 |
| FLPR | 63 | Head | 1 | SN | E | 1 | 7 |
| IL1DL | 64 | Head | 1 | SN | A | 1 | 5 |
| IL1DR | 65 | Head | 1 | SN | A | 1 | 5 |
| IL1L | 66 | Head | 1 | SN | A | 1 | 5 |
| IL1R | 67 | Head | 3 | SN | A | 3 | 5 |
| IL1VL | 68 | Head | 1 | SN | A | 1 | 5 |
| IL1VR | 69 | Head | 3 | SN | A | 3 | 5 |
| IL2L | 70 | Head | 3 | SN | A | 3 | 8 |
| IL2R | 71 | Head | 3 | SN | A | 3 | 4 |
| OLLL | 72 | Head | 2 | SN | A | 2 | 5 |
| OLLR | 73 | Head | 2 | SN | A | 2 | 5 |
| OLQDL | 74 | Head | 2 | SN | A | 2 | 3 |
| OLQDR | 75 | Head | 2 | SN | A | 2 | 3 |
| OLQVL | 76 | Head | 2 | SN | A | 2 | 3 |
| OLQVR | 77 | Head | 2 | SN | A | 2 | 3 |
| RIBL | 78 | Head | 2 | IN | C | 2 | 3 |
| RIBR | 79 | Head | 2 | IN | C | 2 | 3 |
| RICL | 80 | Head | 2 | IN | C | 2 | 8 |
| RICR | 81 | Head | 3 | IN | C | 3 | 4 |
| RID | 82 | Head | 1 | MN | B | 1 | 2 |
| RIFL | 83 | Head | 2 | IN | E | 2 | 3 |
| RIFR | 84 | Head | 2 | IN | E | 2 | 3 |
| RIGL | 85 | Head | 2 | IN | E | 2 | 3 |
| RIGR | 86 | Head | 2 | IN | E | 2 | 3 |
| RIH | 87 | Head | 2 | IN | D | 2 | 3 |
| RIML | 88 | Head | 1 | MN | C | 1 | 1 |
| RIMR | 89 | Head | 1 | MN | C | 1 | 1 |
| RIPL | 90 | Head | 1 | IN | A | 1 | 5 |
| RIPR | 91 | Head | 1 | IN | A | 1 | 5 |
| RIR | 92 | Head | 2 | IN | D | 2 | 3 |
| RIS | 93 | Head | 1 | IN | D | 1 | 1 |
| RIVL | 94 | Head | 2 | MN | C | 2 | 3 |
| RIVR | 95 | Head | 2 | MN | C | 2 | 3 |
| RMDDL | 96 | Head | 2 | MN | D | 2 | 3 |
| RMDDR | 97 | Head | 2 | MN | D | 2 | 3 |
| RMDL | 98 | Head | 2 | MN | C | 2 | 3 |
| RMDR | 99 | Head | 1 | MN | C | 1 | 1 |
| RMDVL | 100 | Head | 2 | MN | C | 2 | 3 |
| RMDVR | 101 | Head | 1 | MN | C | 1 | 1 |
| RMED | 102 | Head | 1 | MN | A | 1 | 5 |
| RMEL | 103 | Head | 2 | MN | A | 2 | 3 |

| | | | | | | | |
|---|---|---|---|---|---|---|---|
| RMER | 104 | Head | 1 | MN | A | 1 | 5 |
| RMEV | 105 | Head | 1 | MN | A | 1 | 5 |
| RMFL | 106 | Head | 2 | MN | D | 2 | 3 |
| RMGL | 107 | Head | 3 | IN | E | 3 | 8 |
| RMGR | 108 | Head | 3 | IN | E | 3 | 4 |
| RMHL | 109 | Head | 3 | MN | D | 3 | 8 |
| RMHR | 110 | Head | 3 | MN | D | 3 | 4 |
| SAADL | 111 | Head | 2 | IN | D | 2 | 3 |
| SAADR | 112 | Head | 2 | IN | D | 2 | 3 |
| SAAVL | 113 | Head | 2 | IN | C | 2 | 3 |
| SAAVR | 114 | Head | 1 | IN | C | 1 | 3 |
| SABD | 115 | Head | 1 | IN | E | 1 | 1 |
| SABVL | 116 | Head | 1 | IN | E | 1 | 1 |
| SABVR | 117 | Head | 1 | IN | E | 1 | 1 |
| SIADL | 118 | Head | 2 | IN | D | 2 | 3 |
| SIADR | 119 | Head | 2 | IN | D | 2 | 3 |
| SIAVL | 120 | Head | 2 | IN | D | 2 | 3 |
| SIAVR | 121 | Head | 2 | IN | D | 2 | 3 |
| SIBDL | 122 | Head | 1 | IN | C | 1 | 2 |
| SIBDR | 123 | Head | 1 | IN | C | 2 | 3 |
| SIBVL | 124 | Head | 1 | IN | D | 1 | 2 |
| SIBVR | 125 | Head | 1 | IN | D | 1 | 3 |
| SMBDL | 126 | Head | 2 | MN | D | 2 | 3 |
| SMBDR | 127 | Head | 2 | MN | D | 2 | 3 |
| SMBVL | 128 | Head | 1 | MN | D | 1 | 3 |
| SMBVR | 129 | Head | 2 | MN | D | 2 | 3 |
| SMDDL | 130 | Head | 1 | MN | D | 1 | 3 |
| SMDDR | 131 | Head | 2 | MN | D | 2 | 3 |
| SMDVL | 132 | Head | 2 | MN | C | 2 | 3 |
| SMDVR | 133 | Head | 2 | MN | C | 2 | 3 |
| URBL | 134 | Head | 2 | IN | A | 2 | 3 |
| URBR | 135 | Head | 2 | IN | A | 2 | 3 |
| URXL | 136 | Head | 3 | SN | B | 3 | 8 |
| URXR | 137 | Head | 3 | SN | B | 3 | 4 |
| URYDL | 138 | Head | 1 | SN | A | 1 | 1 |
| URYDR | 139 | Head | 1 | SN | A | 1 | 1 |
| URYVL | 140 | Head | 1 | SN | A | 1 | 1 |
| URYVR | 141 | Head | 1 | SN | A | 1 | 1 |
| ALML | 142 | Mid body | 1 | SN | F | 1 | 7 |
| ALMR | 143 | Mid body | 1 | SN | F | 3 | 7 |
| AS01 | 144 | Mid body | 1 | MN | E | 1 | 1 |
| AS02 | 145 | Mid body | 1 | MN | G | 1 | 1 |
| AS03 | 146 | Mid body | 1 | MN | G | 1 | 1 |
| AS04 | 147 | Mid body | 1 | MN | G | 1 | 1 |
| AS05 | 148 | Mid body | 1 | MN | G | 1 | 1 |
| AS06 | 149 | Mid body | 1 | MN | G | 1 | 1 |
| AS07 | 150 | Mid body | 1 | MN | G | 1 | 1 |
| AS08 | 151 | Mid body | 1 | MN | G | 1 | 1 |
| AS09 | 152 | Mid body | 1 | MN | G | 1 | 1 |
| AS10 | 153 | Mid body | 1 | MN | G | 1 | 1 |
| AS11 | 154 | Mid body | 1 | MN | H | 1 | 2 |
| AVM | 155 | Mid body | 1 | SN | F | 3 | 7 |

| | | | | | | | |
|---|---|---|---|---|---|---|---|
| DA01 | 156 | Mid body | 1 | MN | E | 1 | 1 |
| DA02 | 157 | Mid body | 1 | MN | G | 1 | 1 |
| DA03 | 158 | Mid body | 1 | MN | G | 1 | 1 |
| DA04 | 159 | Mid body | 1 | MN | G | 1 | 1 |
| DA05 | 160 | Mid body | 1 | MN | G | 1 | 1 |
| DA06 | 161 | Mid body | 1 | MN | G | 1 | 1 |
| DA07 | 162 | Mid body | 1 | MN | G | 1 | 1 |
| DA08 | 163 | Mid body | 1 | MN | H | 1 | 1 |
| DA09 | 164 | Mid body | 1 | MN | H | 1 | 2 |
| DB01 | 165 | Mid body | 1 | MN | E | 1 | 2 |
| DB02 | 166 | Mid body | 1 | MN | E | 1 | 2 |
| DB03 | 167 | Mid body | 1 | MN | G | 1 | 2 |
| DB04 | 168 | Mid body | 1 | MN | G | 1 | 2 |
| DB05 | 169 | Mid body | 1 | MN | G | 1 | 1 |
| DB06 | 170 | Mid body | 1 | MN | G | 1 | 1 |
| DB07 | 171 | Mid body | 1 | MN | G | 1 | 2 |
| DD01 | 172 | Mid body | 2 | MN | E | 2 | 3 |
| DD02 | 173 | Mid body | 2 | MN | G | 2 | 10 |
| DD03 | 174 | Mid body | 2 | MN | G | 2 | 10 |
| DD04 | 175 | Mid body | 1 | MN | G | 1 | 10 |
| DD05 | 176 | Mid body | 2 | MN | G | 2 | 3 |
| PDEL | 177 | Mid body | 1 | SN | F | 1 | 3 |
| PDER | 178 | Mid body | 1 | SN | F | 1 | 3 |
| PVM | 179 | Mid body | 2 | SN | F | 2 | 3 |
| SDQL | 180 | Mid body | 1 | IN | F | 1 | 3 |
| SDQR | 181 | Mid body | 1 | IN | F | 1 | 3 |
| VA01 | 182 | Mid body | 1 | MN | E | 1 | 1 |
| VA02 | 183 | Mid body | 1 | MN | G | 1 | 1 |
| VA03 | 184 | Mid body | 1 | MN | G | 1 | 1 |
| VA04 | 185 | Mid body | 1 | MN | G | 1 | 1 |
| VA05 | 186 | Mid body | 1 | MN | G | 1 | 1 |
| VA06 | 187 | Mid body | 1 | MN | G | 1 | 1 |
| VA07 | 188 | Mid body | 1 | MN | G | 1 | 1 |
| VA08 | 189 | Mid body | 1 | MN | G | 1 | 1 |
| VA09 | 190 | Mid body | 1 | MN | G | 1 | 1 |
| VA10 | 191 | Mid body | 1 | MN | G | 1 | 1 |
| VA11 | 192 | Mid body | 1 | MN | G | 1 | 1 |
| VA12 | 193 | Mid body | 1 | MN | H | 1 | 1 |
| VB01 | 194 | Mid body | 1 | MN | E | 1 | 2 |
| VB02 | 195 | Mid body | 1 | MN | E | 1 | 2 |
| VB03 | 196 | Mid body | 1 | MN | G | 1 | 2 |
| VB04 | 197 | Mid body | 1 | MN | G | 1 | 2 |
| VB05 | 198 | Mid body | 1 | MN | G | 1 | 2 |
| VB06 | 199 | Mid body | 1 | MN | G | 1 | 2 |
| VB07 | 200 | Mid body | 1 | MN | G | 1 | 2 |
| VB08 | 201 | Mid body | 1 | MN | G | 1 | 2 |
| VB09 | 202 | Mid body | 1 | MN | G | 1 | 1 |
| VB10 | 203 | Mid body | 1 | MN | G | 1 | 2 |
| VB11 | 204 | Mid body | 1 | MN | G | 1 | 2 |
| VC01 | 205 | Mid body | 1 | MN | G | 2 | 10 |
| VC02 | 206 | Mid body | 1 | MN | G | 2 | 10 |
| VC03 | 207 | Mid body | 1 | MN | G | 2 | 10 |

| | | | | | | | |
|---|---|---|---|---|---|---|---|
| VC04 | 208 | Mid body | 1 | MN | G | 3 | 10 |
| VC05 | 209 | Mid body | 1 | MN | G | 2 | 10 |
| VD01 | 210 | Mid body | 2 | MN | E | 2 | 3 |
| VD02 | 211 | Mid body | 2 | MN | E | 2 | 3 |
| VD03 | 212 | Mid body | 2 | MN | G | 2 | 3 |
| VD04 | 213 | Mid body | 2 | MN | G | 2 | 10 |
| VD05 | 214 | Mid body | 2 | MN | G | 2 | 10 |
| VD06 | 215 | Mid body | 2 | MN | G | 2 | 10 |
| VD07 | 216 | Mid body | 1 | MN | G | 1 | 10 |
| VD08 | 217 | Mid body | 1 | MN | G | 1 | 1 |
| VD09 | 218 | Mid body | 2 | MN | G | 2 | 3 |
| VD10 | 219 | Mid body | 2 | MN | G | 2 | 3 |
| VD13 | 220 | Mid body | 2 | MN | H | 2 | 3 |
| ALNL | 221 | Tail | 2 | SN | K | 2 | 3 |
| DVA | 222 | Tail | 1 | IN | J | 1 | 2 |
| DVB | 223 | Tail | 1 | MN | J | 1 | 1 |
| DVC | 224 | Tail | 2 | IN | J | 2 | 3 |
| LUAL | 225 | Tail | 1 | IN | K | 1 | 1 |
| LUAR | 226 | Tail | 1 | IN | K | 1 | 2 |
| PDA | 227 | Tail | 1 | MN | H | 1 | 2 |
| PDB | 228 | Tail | 1 | MN | H | 1 | 2 |
| PHAL | 229 | Tail | 2 | SN | K | 2 | 3 |
| PHAR | 230 | Tail | 2 | SN | K | 2 | 3 |
| PHBL | 231 | Tail | 3 | SN | K | 3 | 10 |
| PHBR | 232 | Tail | 3 | SN | K | 3 | 10 |
| PHCL | 233 | Tail | 1 | SN | K | 1 | 1 |
| PHCR | 234 | Tail | 1 | SN | K | 1 | 1 |
| PLML | 235 | Tail | 1 | SN | K | 1 | 1 |
| PLMR | 236 | Tail | 1 | SN | K | 1 | 2 |
| PQR | 237 | Tail | 2 | SN | K | 2 | 3 |
| PVCL | 238 | Tail | 1 | IN | K | 1 | 1 |
| PVCR | 239 | Tail | 1 | IN | K | 1 | 1 |
| PVNL | 240 | Tail | 1 | IN | K | 1 | 2 |
| PVPL | 241 | Tail | 2 | IN | H | 2 | 3 |
| PVPR | 242 | Tail | 2 | IN | H | 2 | 3 |
| PVQL | 243 | Tail | 3 | IN | K | 3 | 4 |
| PVQR | 244 | Tail | 3 | IN | K | 3 | 4 |
| PVR | 245 | Tail | 1 | IN | K | 1 | 2 |
| PVT | 246 | Tail | 2 | IN | H | 2 | 2 |
| PVWL | 247 | Tail | 1 | IN | K | 1 | 1 |
| PVWR | 248 | Tail | 1 | IN | K | 1 | 1 |
